# Supplementary material for: Cradle: Empowering Foundation Agents Towards General Computer Control
Source: arXiv:2403.03186 source file (2024-07-02)
Supplement: Supplementary file 1 [file related_work.tex]

% \section{Related Work}

\subsection{LMM-based Agents for Computer Tasks}
The prosperity of LMMs has broadened the potential of deploying powerful foundation models as autonomous agents for completing complex tasks in various computer applications, such as web navigation~\citep{zhou2023webarena, deng2023mind2web, mialon2023gaia}, software manipulation~\citep{rawles2023android, yang2023appagent,  kapoor2024omniact} and game playing~\citep{wang2023describe, wang2023voyager, ma2023large, xu2024survey}.
While previous LLM-based web agents~\citep{deng2023mind2web, zhou2023webarena, gur2023real, zheng2023synapse} show some promising results in effectively navigating, understanding, and interacting with content on webpages, they usually use raw HTML code and DOM tree as input and interact with the available element IDs, missing the rich visual patterns with key information, like icons, images, and spatial relations. 

Empowered by the advanced LMMs, multimodal web agents~\citep{hong2023cogagent, furuta2023multimodal, yan2023gpt, he2024webvoyager, zheng2024gpt} and mobile app agents~\citep{yang2023appagent,wang2024mobile} have been explored. Instead of HTML source code, they usually take screenshots as input, however, they still need to use the built-in APIs to get the available interactive element IDs to execute corresponding actions.

Similar to web agents, recent works attempt to deploy LLM agents to various complex video games, such as Minecraft~\citep{wang2023describe, wang2023voyager}, Starcraft II~\citep{ma2023large} and Civilization-like game~\citep{qi2024civrealm} with textual observations obtained from internal APIs and pre-defined semantic actions. These domain-specific settings make them struggle with generalizing to other games, let alone websites and other software. Although JARVIS-1\citep{wang2023jarvis} claims to interact with the environment in a human-like manner with the screenshots as input and mouse and keyboard for control, its action space is predefined as a hybrid space composed of keyboard, mouse, and API. 

Though achieving promising results in specific tasks, these methods fail to generalize across various tasks, due to the inconsistent observation and action spaces. This indicates the necessity of the GCC setting, which provides a unified representation of the observation and action spaces for enormous challenging computer tasks.

Concurrent with our work, there are several works~\citep{gao2023assistgui, cheng2024seeclick, niu2024screenagent, zhang2024ufo, wu2024copilot, kapoor2024omniact} aiming to scale agents to more applications (web or not) using screenshots as input and keyboard and mouse operations as output. However, none of them so far control to avoid access or calls to direct APIs or take complex digital games into consideration since they mainly focus on static websites and software, which greatly reduces the need for timeliness and simplifies the setting by ignoring the dynamics between adjacent screenshots, \ie animations, and incomplete action space without considering the duration of the key pressed and different mouse mode. 

\subsection{Decision-Making in Video Games}
Digital games offer very interesting environments for validating agent's various abilities due to their diversity, controllability, safety, and reproducibility, which are also believed to be the most complicated tasks in computer control. 
Atari games~\citep{bellemare2013arcade}, 
Super Mario Bros~\citep{gym-super-mario-bros}, Google Research Football~\citep{kurach2020google}, StarCraft II~\citep{vinyals2019alphastar, samvelyan2019starcraft}, Minecraft~\citep{johnson2016malmo, guss2019minerl, fan2022minedojo} etc, have been the popular environments and benchmarks for reinforcement learning (RL) agents. Besides, RL agents also exhibit impressive performance in Dota II~\citep{berner2019dota}, Quake III~\citep{jaderberg2019human}, Gran Turismo~\citep{wurman2022outracing} and Diplomacy~\citep{meta2022human}. However, to abstract complex computer control, these environments usually simplify the whole action space (\ie keyboard and mouse movement) to pre-defined domain-specific actions, which vary from game to game, exacerbating the poor generalization of RL agents across environments.

Discarding the semantics in the observation and action also leads to low efficiency. 
LLMs enable decision-making agents to leverage semantic information in the environments, which dramatically improves the reasoning ability of agents, Without any training process, Voyager~\citep{wang2023voyager} can efficiently learn to finish long-horizontal complex tasks through code generation. However, it heavily relies on the built-in API tool, Mineflayer, to obtain internal information and execute high-level actions, which are not available in other games. TextStarCraft II~\cite{ma2023large} and CivRealm~\cite{qi2024civrealm} also suffer the same issue. Therefore, closed-source AAA games with rich textual and visual information are rarely to be explored. Pre-trained with videos with action labels, VPT~\citep{baker2022video} manages to output mouse and keyboard control with raw screenshots as input without any additional information. However, collecting videos with action labels is time-consuming and costly, which is difficult to generalize to multiple environments. Another concurrent work, SIMA~\citep{raad2024scaling} trained embodied agents to complete 10-second-long basic tasks over ten 3D video games. Though their results is promising to scale up, they mainly focus on behavior cloning with gameplay data from human experts, resulting in high costs.

In both targeting complex digital games and diverse software applications, our work attempts to explore a new way to efficiently interact with different complex environments in a unified manner and facilitate further data collection. In a nutshell, to our best knowledge, there are currently no agents under the GCC setting, reported to show superior performance and generalization in complex video games or across computer tasks. In this work, we make a preliminary attempt to explore and benchmark diverse environments on this setting, applying our framework to diverse challenging environments under GCC and proposing an approach where any software can be used to benchmark agentic capabilities in it.
